# Supplementary material for: Addressing Corpus Knowledge Poisoning Attacks on RAG Using Sparse Attention
Source: arXiv:2602.04711 source file (2026-08-26)
Supplement: Supplementary file 1 [file Adversarial_Document__Sub_Set_Analysis.tex]

 \section{The Origin of Answers}\label{apn:Adversarial Document (Sub)Set Analysis}

We next study the question of which document subset, from the retrieved set, is the one based on which the answer is generated when using \SDAG{} and \CARG{}.

\paragraph{Towards Dominant Set Selection.}
We consider two types of (sub)sets in the retrieved set:
(i) \textit{Ground Truth Set} (GTS), which consists of documents containing the correct answer; and
(ii) \textit{Adversarial Set} (AS), which consists of the adversarial documents of an attacker.
Note that each set has a corresponding answer (e.g., the correct answer for GTS and the attacker's target incorrect answer for AS).
We define the \textit{dominant set} as the one that includes the majority of documents in the retrieved set.
Exploring alternative dominance criteria or additional set definitions is left for future work.
We define the \textit{dominant-set-based generation} of a set as the proportion of cases (i.e., questions) in which the RAG output corresponds to the answer of the dominant set, out of all instances in which the set is dominant.
We focus on GTS analysis because AS is never dominant in our experimental setting, as it contains only a single document.



Table~\ref{tab:dominant_cluster_across_datasets} presents the dominant-set-based generation of GTS for \SDAG{} and \CARG{} using E5.
In all cases, \SDAG{} achieves a higher dominant-set-based generation than \CARG{}, with statistically significant improvements in most cases.
This finding attests to the fact that \SDAG{} steers the generator to attend more frequently to the GTS when it is dominant than \CARG{}, which helps to explain \SDAG{}'s superiority over \CARG{}. 
These observations provide insight into the underlying mechanism of \SDAG{}, which steers the RAG towards deriving answers from a dominant (sub)set of documents.



\input{tables/dominant_cluster_by_datasets}




 
\paragraph{Adversarial Document (Sub)Set Analysis.} Above, we show that \SDAG{} steers the generator to attend more frequently to dominant subsets of documents in the retrieved set that contain the correct answer to a question. We now turn to study whether this finding holds for subsets composed of adversarial documents.
Specifically, we analyze the dominant-set-based generation of AS in the multiple-adversarial-document \nonOracle{} setting. 
Note that in a single-document setting, the retrieved set includes one adversarial document at most (i.e., the AS is never dominant); therefore, we inject a pool of five adversarial documents into the corpus.
To ensure the existence of the two sets defined above for informative dominant set analysis, we exclude questions where the retrieved set consists only of adversarial documents.

Table~\ref{tab:adversarial_dominant_cluster_analysis} reports the dominant-set-based generation of AS for \SDAG{} and \CARG{} using E5.
In contrast to the GTS analysis presented in Section~\ref{sec:RQ2}, we do not observe consistent differences in dominant-set-based generation of AS when comparing \SDAG{} with \CARG{}.
In fact, in all cases, the dominant-set-based generation of \SDAG{} and \CARG{} is statistically significantly indistinguishable. 
This finding indicates that \SDAG{}'s more frequent generator steering towards dominant GTS than \CARG{}  observed in Section~\ref{sec:RQ2} does not hold for subsets of adversarial documents.



\input{tables/adversarial_dominant_cluster_analysis}
