# Supplementary material for: Addressing Corpus Knowledge Poisoning Attacks on RAG Using Sparse Attention
Source: arXiv:2602.04711 source file (2026-08-26)
Supplement: Supplementary file 2 [file attack_strategies.tex]

\input{tables/additional attack strategies (contriever and BM25)}

\section{\SDAG{} Evaluation Under Different Attack Strategies}
In this section, we evaluate \SDAG{} using Qwen and Mistral as generators on the attack strategies defined in Section~\ref{sec:threat Model}: \textit{Random}, \textit{Near}, and \textit{Far}.
As in \SDAG{} evaluation in Section~\ref{sec:RQ1}, where we evaluate \SDAG{} on those attack strategies using Llama as generator, we consider the \oracle{} single-adversarial-document setting.
